# Supplementary material for: ZerO Initialization: Initializing Neural Networks with only Zeros and Ones
Source: arXiv:2110.12661 source file (2022-11-04)
Supplement: Supplementary file 1 [file hadamard.tex]

\section{Hadamard Transform}

\textbf{to be changed}

The reason for the degeneracy is that the skip connection $\mI^{1}$ with zero padding is only able to map the input $\vx$ into \emph{a low-dimensional subspace} of $\va^{1}$. As illustrated in Figure \ref{fig:symmetry}, when initializing all the weights to zero, $\mI^{1}$ maps the single dimension $\vx$ to a horizontal line (dashed line) in the two-dimensional space. Because this subspace is aligned with the standard basis, its linear dimension is invariant under application of the Relu, or any component-wise nonlinearity. As the activations $\va^{1}$ stay in a 1-dimensional subspace $\operatorname{span}$, its associated derivatives stay in such a subspace as well. This eventually causes the zero-initialized weights $W^{1}$ to be updated into a low-dimensional space, as they solely depend on the low-dimensional derivatives. 

% option: mention that linearity decouples the linear correlation
% Is this a good way to say nonlinearity breaks linear correlation
% Nonlinear neural networks have more expressive power than linear neural networks mostly because the nonlinearity decouples the linear correlation between neurons. However, nonlinearity does not break the linear correlation when neurons have the exact same values before feeding into nonlinearity, such as $\vh^{1}_3$ and $\vh^{1}_4$ where $\vh^{1}$ is the hidden space of the first layer in Figure \ref{fig:symmetry}. This is because the neurons still receive the same value after the nonlinearity: $\phi(\vh^{1}_3) = \phi(\vh^{1}_4)$, as the $\vh^{1}_3$ and $\vh^{1}_4$ are aligned with each other over the coordinate basis of the nonlinearity. Therefore, it is important to break such an alignment to unleash the power of nonlinearity. 

To ensure that the first hidden space receives high-dimensional activations $\va^{1}$, we propose to apply a \emph{Hadamard transform} $\mH^{1}$ after $\mI^{1}$ to spread the information into a new space. 

The Hadamard transform is an example of the generalized family of Fourier transforms that performs an orthogonal linear operation on $2^{m}$ real numbers \citep{pratt_hadamard_1969}. It consists of a Hadamard matrix and a normalization factor. A Hadamard matrix is defined as follows:
\begin{restatable}[Hadamard matrix]{definition}{hadamardmatrix}\label{def:hadamardmatrix}
    For any Hadamard matrix $\mH_{m} \in \sR^{2^{m} \times 2^{m}}$ where $m$ is a positive integer, we define $\mH_{0} = 1$ by the identity, and the matrix with large $m$ is defined recursively:
    \begin{equation*}
        \mH_{m}= \left(\begin{array}{cc}
        \mH_{m-1} & \mH_{m-1} \\
        \mH_{m-1} & -\mH_{m-1}
        \end{array}\right)\quad = \quad
        {\tiny
        \begin{pmatrix}    
            1 & 1 & 1 &  1 & \dots \\
            1 & -1 & 1 &  -1 & \dots \\
            1 & 1 & -1 & -1 & \dots \\
            1 & -1 & - 1 & 1 & \dots \\
            \vdots & \vdots & \vdots &\vdots &\ddots 
        \end{pmatrix}}
        \in \sR^{2^{m} \times 2^{m}}.
    \end{equation*}
\end{restatable}
We rescale the Hadamard matrix by $2^{-(m-1)/2}$, resulting in the orthonormal Hadamard transform. 
The Hadamard transform rotates the standard basis into a new basis, such that each element of the new basis is equally weakly aligned with every element of the standard basis. 
For example, in a two-dimensional space, the Hadamard transform rotates the standard basis by an angle of $45$ degree, as illustrated in Figure \ref{fig:symmetry} \footnote{We use a column-order-reversed Hadamard matrix in the example to simplify the presentation. This is equivalent to using a standard Hadamard matrix with order-reversed $\mI^{1}$, without affecting our conclusions.}.

% may need to extend the discussion about the power of nonlinearity.
When applying component-wise nonlinearities to the spaces spanned by the elements of this basis, their linear dimension increases. In our example, after applying the Hadamard matrix $\mH^{1}$ to $\mI^{1}\vx$, it forms a new space that is not aligned with the standard basis. Under the application of the Relu, the new space (i.e., $\mH^{1}\mI^{1}\vx$) is spread into a 2-dimensional $\operatorname{span}$ in $\va^{1}$, which ensures that neither $\va^{1}_{0}$ nor $\va^{1}_{1}$ stay at zero forever. Therefore, with the Hadamard transform, the activation $\va^{1}_{1}$ can propagate the non-zero signals to the next layer. This ensures the derivatives of $\mW^{2}_{1,1}$ and $\mW^{2}_{0,1}$ to be non-zero, and thus breaks the training degeneracy.

% may generalize it to a broad setting
