# Supplementary material for: ZerO Initialization: Initializing Neural Networks with only Zeros and Ones
Source: arXiv:2110.12661 source file (2022-11-04)
Supplement: Supplementary file 2 [file network_pruning.tex]

\section{Network Pruning}

As shown in Figure \ref{fig:linear_results}, the network trained by ZerO has a weight variance significantly smaller than the networks trained by random initialization methods. Because the weights that are close to zero usually have smaller effects on the network, they can be pruned to increase the network sparsity while preserving the prediction performance. For ZerO initialization, as most of the weights are extremely close to zero even after training, this motivates us to discover whether ZerO helps to generate sparse networks through pruning. 

To verify our hypothesis, we apply a standard magnitude-based pruning for the trained networks initialized with different initializers. We then evaluate the test accuracy of the pruned networks. The magnitude-based pruning method prunes a portion of weights with the lowest magnitudes in each layer. We use the network described in Appendix \ref{appendix:linear_design} for MNIST and ResNet-18 for CIFAR-10. Standard ResNet-18 is adopted for Kaiming and Xavier initializers for better accuracy, and ResNet-18 (AugSkip) is applied for ZerO initializer. 

As shown in Figure \ref{fig:pruned_networks}, compared to Kaiming and Xavier initializers, the networks trained with ZerO initializer can be pruned more aggressively while preserving the test accuracy. Because the state-of-the-art pruning methods adopt standard random initializers by default, we believe ZerO would be a powerful replacement that improves the pruning performance. 

\begin{figure}[h!]
    \centering
    % \vskip -0.3in
    \begin{minipage}{0.5\textwidth}
    \centering
    \includegraphics[width=0.8\textwidth]{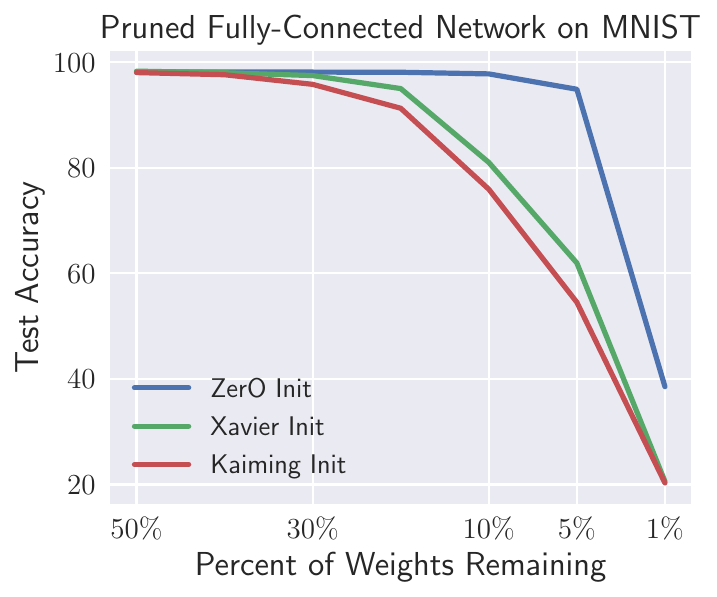}
    \end{minipage}%
    \begin{minipage}{0.5\textwidth}
    \centering
    \includegraphics[width=0.8\textwidth]{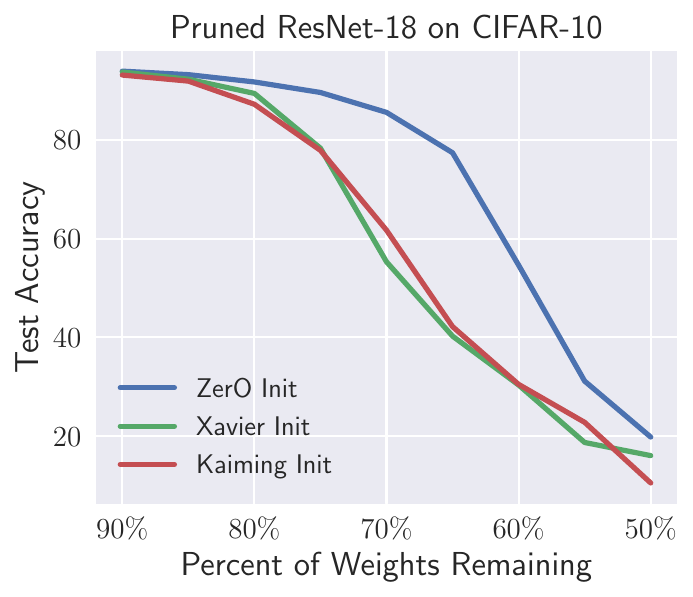}
    \end{minipage}
    % \vskip -0.13in
    \caption{Test accuracy of the pruned networks trained with various initialization methods.}
    \label{fig:pruned_networks}
    % \vskip -0.15in
\end{figure}
