# Supplementary material for: ZerO Initialization: Initializing Neural Networks with only Zeros and Ones
Source: arXiv:2110.12661 source file (2022-11-04)
Supplement: Supplementary file 3 [file non_bn.tex]

\section{Training without normalization}
We also evaluate the ability of ZerO to remove batch normalization during training. We use the residual blocks that replace batch normalization, as illustrated in Figure \ref{fig:structure}. We compare various initialization methods using ResNet-50 on ImageNet, including a recent normalization-free method called Fixup \citep{<fixup>}. As the training without batch normalization usually suffers from overfitting, we apply a stronger regularization technique Mixup \citet{zhang_mixup_2018}, which is the same as the training setting in \citep{<fixup>}. The Mixup coefficient is tuned for each setting, and we train ResNet-50 for $90$ epochs. 
We find that training with ZerO is stable with default hyperparameters such as a learning rate of $0.1$. This is not always the case for training without normalization, as the training with Kaiming initialization fails when using $0.1$ as the learning rate.

As shown in Table \ref{tab:non_bn_results}, without batch normalization, ZerO achieves significantly better results than standard random initialization such as Xavier and Kaiming. We observe that ZerO is slightly worse than Fixup, which is likely due to the difference in the speed of convergence. When we train both models for 180 epochs, the gap is largely reduced from 0.7\% to 0.2\%. 
\begin{table}[h]
\centering

\begin{tabular}{lccc}
\toprule
\textbf{Method}               & \textbf{Batch Normalization}         & \textbf{Large Learning Rate}          & \textbf{Test Error} \small{(mean $\pm$ std)} \\
\midrule
Kaiming Init            & \cmark & \cmark &        $23.46 \pm 0.07$            \\
Kaiming Init + Mixup           & \cmark & \cmark &        $23.16 \pm 0.09$           \\
\hline
\small{\textit{(Mixup enabled)}} &&& \\
\textbf{ZerO Init}    & \xmark & \cmark &        $24.52 \pm 0.06$            \\
Fixup Init  & \xmark & \cmark &        $23.85 \pm 0.10$            \\
Kaiming Init & \xmark & \xmark &        $29.91 \pm 0.12$            \\
Xavier Init & \xmark & \cmark &        $25.89 \pm 0.11$            \\
\bottomrule
\end{tabular}
\caption{Benchmarking ResNet-50 without batch normalization on ImageNet}
\label{tab:non_bn_results}
\end{table}
