# Supplementary material for: ZerO Initialization: Initializing Neural Networks with only Zeros and Ones
Source: arXiv:2110.12661 source file (2022-11-04)
Supplement: Supplementary file 4 [file proofs-x.tex]

\section{Proofs}

\begin{definition}[Residual network]
    \label{def:non_linear_residual_network}
        We define a non-linear residual network $\funcF_{n}(\vx)$ as follows:
        $$\funcF_{n}(\vx) = \relu \circ (\mW_{L} + \mI_{L}) ... \circ \relu \circ (\mW_{l} + \mI) ... \circ \relu \circ (\mW_{1} + \mI_{1}) \vx,$$ 
        where $L \geq 2$. Let $\mW_{L},\mI_{L} \in \sR^{n_y \times n_h}$ and $\mW_{1},\mI_{1} \in \sR^{n_h \times n_x}$, where $\mI_{L}$ and $\mI_{1}$ are adaptive identity mappings defined in Equation~\ref{eq:adaptive_identity}. For any layer $l$ except $1$ and $L$, we assume $\mW_{l} \in \sR^{n_h \times n_h}$ and we let $I \in \sR^{n_h \times n_h}$ to be the standard identity mapping. We denote $\relu$ as any nonlinearity.
\end{definition}

\begin{definition}[Hadamard-based residual network]
    \label{def:hadamard_non_linear_residual_network}
        A Hadamard-based residual network $\funcF_{h}(\vx)$ is defined as follows:
        $$ \funcF_{h}(\vx) = \relu \circ (\mW_{L} + \mI_{L}) \mH^{\top} ... \circ \relu \circ (\mW_{l} + \mI) ... \circ \relu \circ \mH (\mW_{1} + \mI_{1}) \vx,$$
        where $\mH \in \sR^{n_h \times n_h}$ denotes a normalized Hadamard matrix, and the rest follows Definition~\ref{def:non_linear_residual_network}
\end{definition}

\begin{restatable}{theorem}{main_thm}
    We have the following results for zero and random initialization:
    \begin{enumerate}[label={\upshape(\roman*)}]
        \item For a standard residual network $\funcF_{n}(\vx)$, when initializing the network at zero, every matrix $\mW_{l}$ follows a rank constraint during the entire training, such that:
        \begin{equation}
            % \label{eq:low_rank_non_linear}
            \rank(\mW_{l}) \leq \min (n_x, n_y) \quad \text{for } l \in 1,...,L.
        \end{equation}
        \item For a Hadamard-based residual network $\funcF_{h}(\vx)$, when initializing the network at zero, there exists a matrix $\mW_{l}$ that breaks the above rank constraint after the first iteration, such that:
        $$\rank(\mW_{l}) > \min (n_x, n_y) \quad \text{for } l \in 1,...,L.$$
        \item For either $\funcF_{n}(\vx)$ or $\funcF_{h}(\vx)$, when initializing the network randomly, every matrix $\mW_{l}$ reaches its maximum rank at the initialization, almost surely.
    \end{enumerate}
\end{restatable}

\begin{remark}
    Some remarks left.
\end{remark}

In the following, we will rigorously describe and prove the claims in Theorem~\ref{thm:main_thm}. Each claim is described in a seperate theroem below.

\begin{restatable}{theorem}{low_rank_non_linear}[Claim 1 in Theorem~\ref{thm:main_thm}]
    \label{thm:low_rank_non_linear}
    Consider a non-linear residual network defined in Definition~\ref{def:non_linear_residual_network}. When initializing every matrix $\mW_{l}$ at zero and training the function using gradient descent, at any iteration $t$, we have that:
    \begin{equation}
        % \label{eq:low_rank_non_linear}
        \rank(\mW_{l}^{t}) \leq \min (n_x, n_y) \quad \text{for } l \in 1,...,L.
    \end{equation}
\end{restatable}

\begin{proof}
    When $n_h \leq \min(n_x, n_y)$, the rank constraint in Equation~\ref{eq:low_rank_non_linear} is satisfied trivially. We then move our focus on a more common case, where the large hidden dimension exsists: $n_h > \min(n_x, n_y)$.

    In this case, the initial derivative for each matrix is derived as follows:
    \begin{lemma}
        \label{lemma:init_gradient_non_linear_large_width}
        When $n_h > n_x,n_y$, the initial derivatives become:
        \begin{equation*}
        \grad{\loss}{\mW_{1}^0} = 
        \begin{pmatrix*}
            \Lambda \\
            \bm{0} \\
        \end{pmatrix*}
        \in \sR^{n_h \times n_x},
        \quad
        \grad{\loss}{\mW_{l}^0} = 
        \begin{pmatrix*}
            \Lambda & \bm{0} \\
            \bm{0} & \bm{0} \\
        \end{pmatrix*}
        \in \sR^{n_h \times n_h},
        \quad
        \grad{\loss}{\mW_{L}^0} =
        \begin{pmatrix*}
            \Lambda & \bm{0} \\
        \end{pmatrix*}
        \in \sR^{n_y \times n_h},
        \end{equation*}
        where $\Lambda = \sum_{\mu=1}^{P} \relu^{\prime}(\vz^{\mu}) \odot (\vz^{\mu} - \vy^{\mu}) \vx^{\mu^{T}} \in \sR^{n_y \times n_x}$. We let $\vz^{\mu} = \mI_{L} \circ \relu \circ \mI_{1} \vx^{\mu}$ and $l \in 2,...,L-1$. We denote $\bm{0}$ as a zero vector or a zero matrix depending on the dimensionality. Let $\odot$ represent an element-wise multiplication.
    \end{lemma}
    As shown in the above lemma, in the initial derivative of each matrix, the elements are zero except for a sub-matrix determined by $\Lambda$. Because the parameters with zero initial derivatives stall at zero during the entire training, the rank constraint in Theorem~\ref{thm:low_rank_non_linear} is satisfied.
\end{proof}

\begin{restatable}{theorem}{breaking_low_rank}[Claim 2 in Theorem~\ref{thm:main_thm}]
    \label{thm:breaking_low_rank}
    Consider a non-linear residual network with Hadamard transforms (Definition~\ref{def:hadamard_non_linear_residual_network}) $\funcF_{h}(\vx)$. When initializing every matrix $\mW_{l}$ at zero and training the function using gradient descent, there exists a matrix $\mW_{l}$ after the first iteration, such that: 
    $$\rank(\mW_{l}^{1}) > \min (n_x, n_y).$$
\end{restatable}

\begin{proof}
    We focus on a particular intermediate layer $l$ in the network $\funcF_{h}(\vx)$, where $l$ is not 1 or $L$, such that:
    \begin{align*}
        \vx_{1} &= (\mW_{1} + \mI_{1}) \vx \\
        \vz_{1} &= \relu (\vx_{1}) \\
        ... \\
        \vx_{l} &= (\mW_{l} + \mI) \vz_{l-1} \\
        \vz_{l} &= \relu (\vx_{l}) \\
        ... \\
        \vx_{L} &= (\mW_{L} + \mI_{L}) \vz_{L-1} \\
        \funcF_{h}(\vx) &= \vz_{L} = \relu (\vx_{L}) \\
    \end{align*}

    The derivative of each layer $l$ is:
    $$\grad{\loss}{\mW_{l}} = \sum_{\mu=1}^{P} \grad{\loss}{\vx_{l}^{\mu}} \vz_{l-1}^{\mu^{\top}} $$

    This is a sum of rank-1 matrices. We define a general form of the problem as follows:
    $$\mM = \sum_{\mu=1}^{N} \va^{\mu} \vb^{\mu^{\top}}.$$
    We have the following proposition regarding the rank of $\mM$:
    \begin{proposition}
        \label{prop:rank_sum_rank_1}
        Consider a matrix $\mM$ to be a sum of vector outer products:$\mM = \sum_{\mu=1}^{N} \va^{\mu} \vb^{\mu^{\top}}.$
        We define $\mV$ and $\mU$ as two vector spaces where $\dim (\mV) = n_v$ and $\dim (\mU) = n_u$, respectively. Let $\va^{\mu} \overset{\mathrm{iid}}{\sim} U(\mV)$ and $\vb^{\mu} \overset{\mathrm{iid}}{\sim} U(\mU)$ for any $\mu \in \{1,\dots,N\}$, where $U(\mV)$ and $U(\mU)$ denotes the uniform distributions over the vector space $\mV$ and $\mU$. We have that:
        $$ \lim_{N \to \infty} \rank (M) = \min (n_v, n_u) $$
    \end{proposition}
    Briefly describe and prove this proposition.

    We then go back to measure the rank of $\grad{\loss}{\mW_{l}}$. To ensure $\rank(\grad{\loss}{\mW_{l}}) > \min (n_x, n_y)$, we need to ensure that $\grad{\loss}{\vx_{l}^{\mu}}$ is contained within a vector space $\mV$ with $\dim (\mV) > n_y$, and $\vz_{l-1}^{\mu}$ is contained within a vector space $\mU$ with $\dim (\mV) > n_x$.

    To show this, we need to introduce the following proposition:
    % To-Do: replace \vx using a more general term
    \begin{proposition}
        \label{prop:nonlinar_expand_dim}
        For any $\vx \in \sR^{n_x}$, $\relu \mH \mI_{1} \vx$ lies in a vector space $\mV$ with $\dim (\mV) > n_x$.
    \end{proposition}

    We can prove this proposition by deduction. Assume $\vx \in \sspan (\ve_{1})$ where $\ve_{1}$ a coordinate vector, which indicates $\vx$ lives in a 1-dimensional space. Let $\vx = \alpha \cdot \ve_{1}$ for a scalar $\alpha \neq 0$. It's easy to see that:
    \begin{equation*}
        \relu \mH \mI_{1} \vx =
        \begin{cases}
            \alpha \relu (\mH \mI_{1} \ve_{1}) & \text{ for } \alpha > 0, \\
            \alpha \relu (-\mH \mI_{1} \ve_{1}) & \text{ for } \alpha < 0.
        \end{cases}
    \end{equation*}
    Because $\relu (\mH \mI_{1} \ve_{1})$ and $\relu (-\mH \mI_{1} \ve_{1})$ are linearly independent, this ensures that the operation $\relu \circ \mH \mI_{1}$ maps $\vx$ from a 1-dimensional space to a 2-dimensional space. 

    % QQQ: needs to rethink the derivation here, more rigorously. 
    Also, if $\vx \in \sspan (\ve_{1}, \ve_{2})$, $\relu \mH \mI_{1} \vx$ lies in a 4-dimensional space. By deduction, we can show that $\relu \circ \mH \mI_{1}$ always maps $\vx$ to a higher dimensional space. Thus, for any $\vz^{0}_{l-1} \vx \in \sR^{n_x}$, $\relu \mH \mI_{1} \vx$ lies in a vector space $\mV$ with $\dim (\mV) > n_x$. 
    
    Similarly, we can show that $\grad{\loss}{\vx_{l}}$ lies in a vector space $\mU$ with $\dim (\mU) > n_y$. By Proposition~\ref{prop:rank_sum_rank_1}, we know that $\rank (\grad{\loss}{\mW_{l}}) > \min(n_x, n_y)$ holds when number of samples $P$ is large enough. Thus, after the first iteration, $\mW_{l}^{1}$ breaks the rank constraint as well. 
    
\end{proof}

\begin{restatable}{theorem}{full_rank_non_linear_random}[Claim 3 in Theorem~\ref{thm:main_thm}]
    \label{thm:full_rank_non_linear_random}
    For either $\funcF_{n}(\vx)$ or $\funcF_{h}(\vx)$, when initializing it randomly based on a Gaussian distribution $\mathcal{N}(\mu, \sigma^{2})$, at initialization, every matrix $\mW_{l}^{t}$ reaches its maximum rank almost surely, for $l \in 1,...,L$.
\end{restatable}

\begin{proof}
    We want to show that for any matrix $\mW \in \sR^{M \times N}$, if each entry is sampled from a Gaussian distribution $\mathcal{N}(\mu, \sigma^{2})$, then $\mW$ will achieve full-rank (i.e., $\rank(\mW) = \min (M,N)$) with probability of one. 
    
    Assume $M \geq N$ without losing generality. We want to prove the following statement:
    $$\prob(\rank(\mW) < N) = 0.$$
    Let $\{\vv_{i}\}$ be columns of $\mW$, where $\vv_{i} \in \sR^{M}$ for $i \in \{1,...,N\}$. We denote $P_{i}$ as the probability of the event where a column $\vv_{i}$ is linearly dependent on the rest of the columns $\{\vv_{j}\}$, for $j \neq i$. If $\mW$ does not reach the full-rank, then there exsists at least a column that is linearly dependent on the rest of the columns. Thus, by the union bound, we know that:
    $$\prob(\rank(\mW) < N) \leq \sum_{i=1}^{N} P_{i}.$$
    For each $P_{i}$, it is equivalent to the probability of the event where $\vv_{i} \in \sS = \text{span}(\vv_{1},...,\vv_{j})$, for $j \neq i$. Since $\sS$ at most has $N-1$ dimension, it is a subspace of $\sR^{M}$. Because each entry of $\vv_{i} \in \sR^{M}$ is sampled from a continuous Gaussian distribution, the probability that $\vv_{i}$ fails into a low-dimensional subspace $\sS$ is zero. Thus, $P_{i} = 0$ for any $i \in \{1,...,N\}$, and $\prob(\rank(\mW) < N) = 0$. We can conclude that $\mW$ reaches the full-rank almost surely.

\end{proof}

% \begin{lemma}
%     The derivative of each matrix $W^{l}$ in linear residual network defined in Definition~\ref{def:linear_residual_network} is:
%     \begin{equation*}
%         \begin{split}
%             \grad{\loss}{\mW^1} &= \sum_{\mu=1}^{P} ((\mW^L + \mI^{L}) \,...\, (\mW^2 + \mI))^{\top} \, (\funcF(\vx^{\mu}) - \vy^{\mu}) \, \vx^{\mu^{\top}}, \\
%             %to-do think about whether we should exclude l=2 and l=L-1 as well
%             \grad{\loss}{\mW^l} &= \sum_{\mu=1}^{P} ((\mW^L + \mI^{L}) \,...\, (\mW^{l+1} + \mI))^{\top} \, (\funcF(\vx^{\mu}) - \vy^{\mu}) \, ((\mW^{l-1} + \mI) \,...\, (\mW^{1} + \mI^{1}) \, \vx^{\mu})^{\top} \quad \text{for } l \in 2,...,L-1, \\
%             \grad{\loss}{\mW^L} &= \sum_{\mu=1}^{P} (\funcF(\vx^{\mu}) - \vy^{\mu}) \, ((\mW^{L-1} + \mI) \,...\, (\mW^{1} + \mI^{1}) \, \vx^{\mu})^{\top}.
%         \end{split}
%     \end{equation*}
% \end{lemma} 
