# Supplementary material for: ZerO Initialization: Initializing Neural Networks with only Zeros and Ones
Source: arXiv:2110.12661 source file (2022-11-04)
Supplement: Supplementary file 5 [file x-correlation_mesurements.tex]

\begin{figure}[t!]
    \centering
    \vskip -0.3in
    \begin{minipage}{0.5\textwidth}
    \centering
    \includegraphics[width=0.8\textwidth]{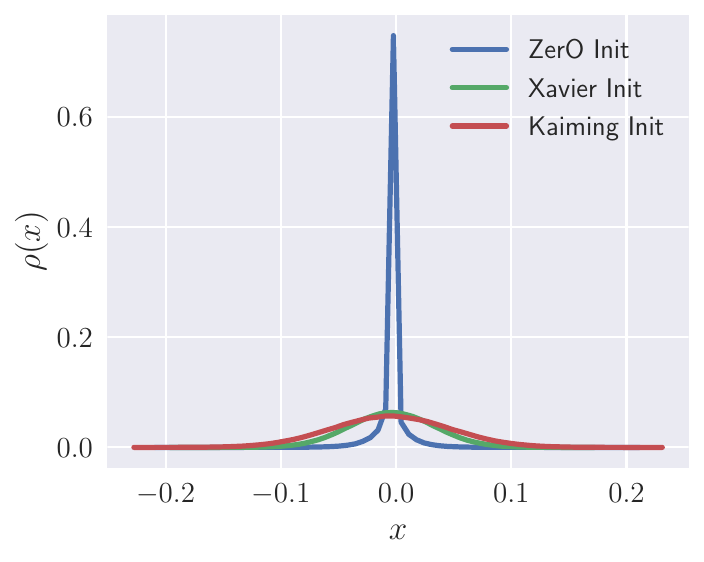}
    \end{minipage}%
    \begin{minipage}{0.5\textwidth}
    \centering
    \includegraphics[width=0.8\textwidth]{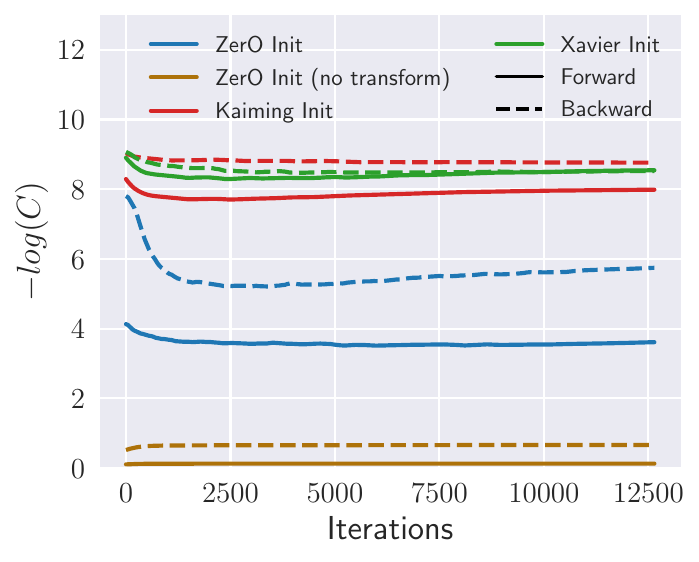}
    \end{minipage}
    \vskip -0.13in
    \caption{\textbf{Left:} final weight distributions. \textbf{Right:} weight correlations during training. Each setting achieves 98\% test accuracy on MNIST dataset except for ZerO Init (no transform). }
    \label{fig:linear_results}
    \vskip -0.15in
\end{figure}

\textbf{to be changed with rank verification experiments}

To verify the phenomenon explained above empirically, we train a fully connected residual network on the MNIST dataset to check the existence of the degeneracy and measure the weight distribution \citep{lecun_gradient-based_1998}. 
Our network has three layers with hidden dimensions larger than the input dimension. The details of our setting are introduced in the appendix.

We use empirical weight correlations as a proxy to verify the existence of the degeneracy, which is similar to the measurement conducted by \citet{<feature_diversity>}. 
High weight correlations indicate that degeneracy may exist. 
For each weight matrix, we measure the correlations between row vectors and column vectors, respectively. 
For example, given a $M \times N$ weight matrix $\mW$, we define forward correlations (between rows) $C_f$ and backward correlations (between columns) $C_b$ as follows:
\begin{equation*}
    \begin{split}
        C_f = \frac{1}{M(M-1)} \sum_{i}^{M} \sum_{i \neq j}^{M} \frac{\mW_{i,:} \cdot \mW_{j,:}}{\norm{\mW_{i,:}}_2 \, \norm{\mW_{i,:}}_2}, \\
        C_b = \frac{1}{N(N-1)} \sum_{i}^{N} \sum_{i \neq j}^{N} \frac{\mW_{:,i} \cdot \mW_{:,j}}{\norm{\mW_{:,i}}_2 \, \norm{\mW_{:,j}}_2},
    \end{split}
\end{equation*}
where $A \cdot B$ denotes a dot product of vectors. We measure the weight correlations for the zero-initialized network with or without the Hadamard transform, and compare them with popular initialization methods proposed by \citet{<xavier>,<kaiming>}. As shown in Figure \ref{fig:linear_results}, the Hadamard transform largely decouples the weight correlations compared to the network without the transform, which suggests that the Hadamard transform avoids the problem of training degeneracy.

% may discuss it - the effect of sample correlation
%We also observe that the random initialization methods achieve smaller correlations than ours. We believe this is because, in our setting, the weights inherit the correlations from the samples, as they solely depend on the sample diversity at initialization. Although the additional sample correlations do not affect the final accuracy, it is an interesting direction to discover the effect of these correlations during training, and we will investigate it in the future.

% weight distribution
In addition, we measure the final weight distributions over various initialization methods. As shown in Figure \ref{fig:linear_results}, the weight variance generated by our initialization is significantly lower than the variances generated by randomized methods. 
We believe that the fact that most of our weights are close to zero may help to train sparse neural networks with techniques such as weight pruning\citep{han_heep_2016}.

% point out where we need to initialize as one, for batch-norm layers

%Previous methods to break the symmetric: random weight initialization, dropout or GPU arithmetics

% Compare those methods based on the measurements
