# Supplementary material for: ZerO Initialization: Initializing Neural Networks with only Zeros and Ones
Source: arXiv:2110.12661 source file (2022-11-04)
Supplement: Supplementary file 6 [file additional_discussion.tex]

\section{Additional discussions}

\subsection{Zero-initialized linear model}
\label{sec:zero_linear}
